# Supplementary material for: Observation of strangeness enhancement with charmed mesons in high-multiplicity $p\mathrm{Pb}$ collisions at $\sqrt {s_{\mathrm{NN}}}=8.16\,$TeV
Source: arXiv:2311.08490 source file (2024-09-04)
Supplement: Supplementary file 3 [file appendix1.tex]

\clearpage
\section*{Appendices}
\label{sec:Appendix}

\appendix

%The double differential cross-sections for prompt \Ds and \Dp mesons in both forward and backward rapidities are shown in Fig. \ref{fig:cross_section_Ds} and Fig. \ref{fig:cross_section_Dp}.

\begin{figure}[tb]
    \begin{center}
    \includegraphics[width=1.0\linewidth]{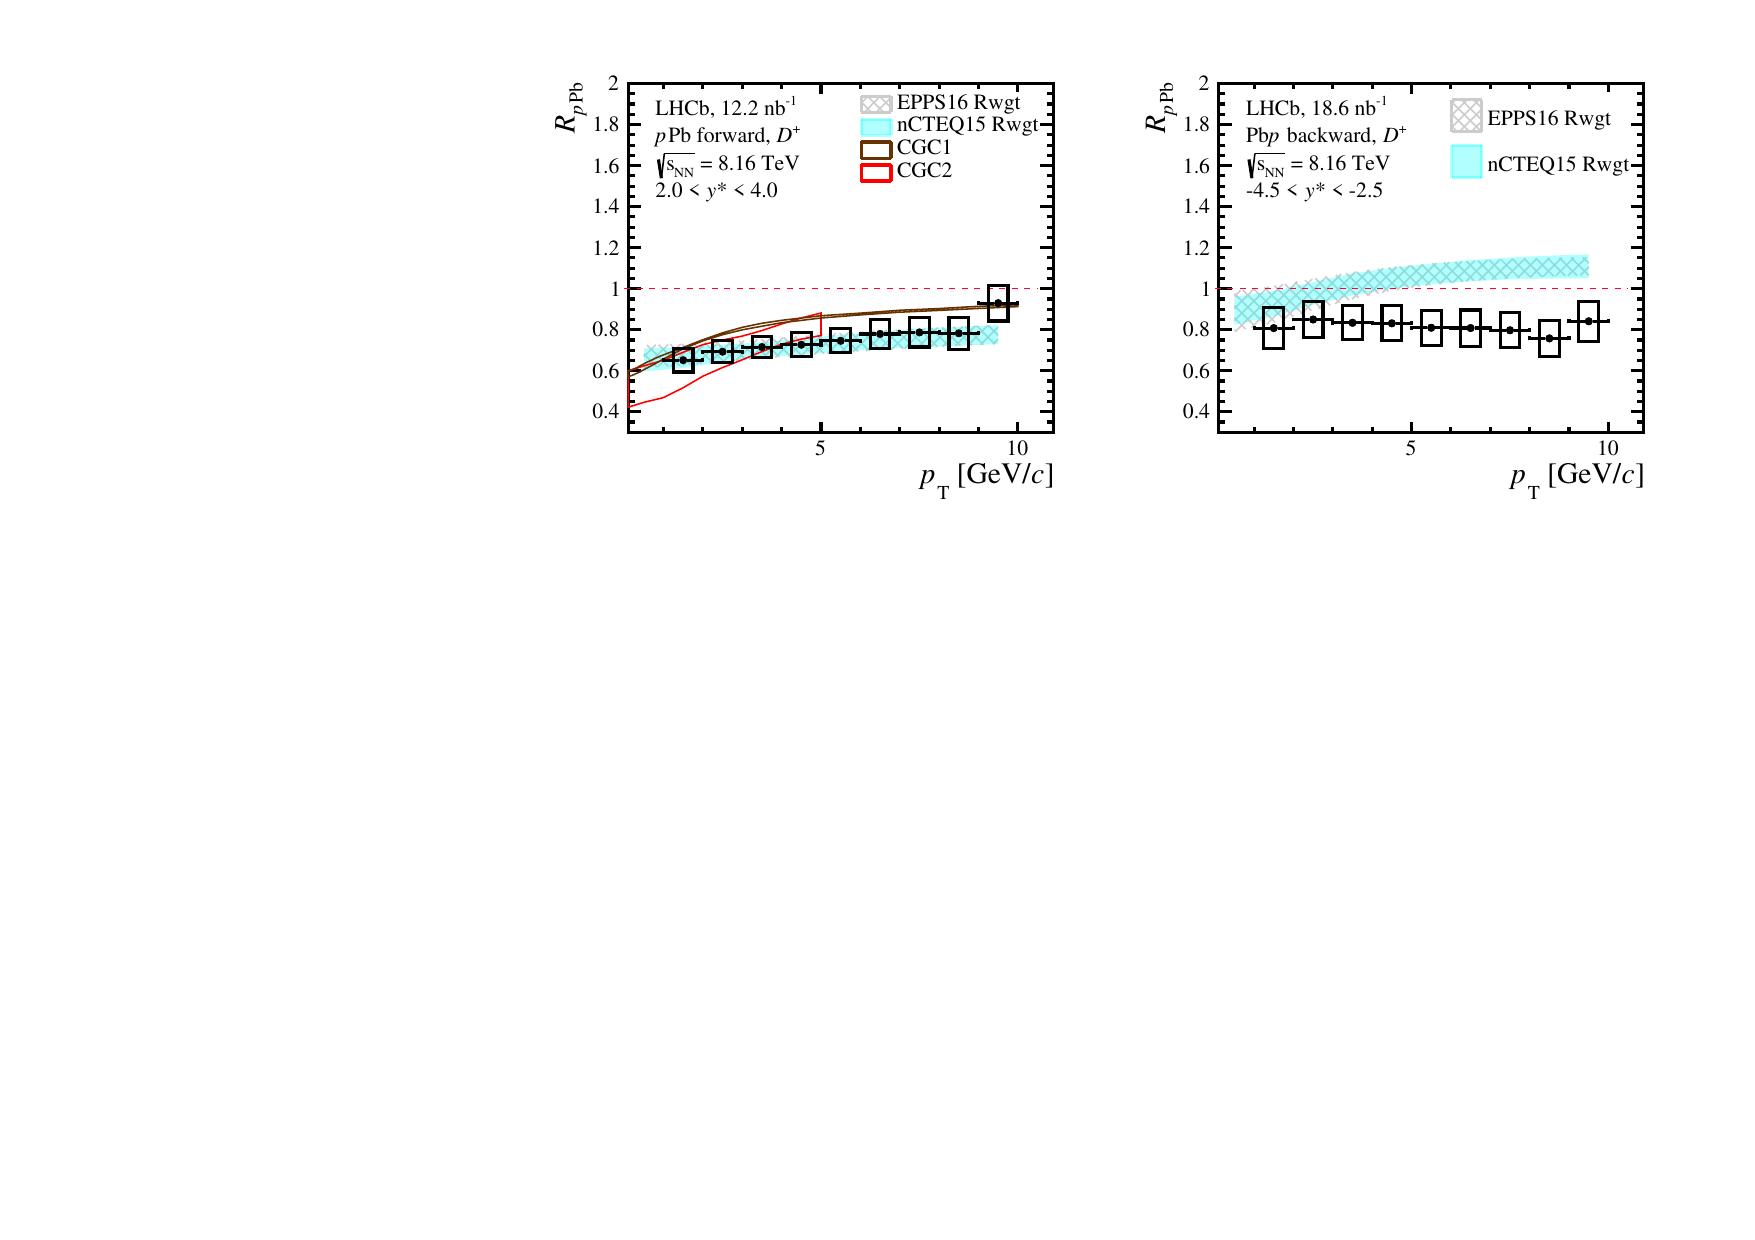}
    \vspace*{-0.5cm}
    \end{center}
    \caption{Nuclear modification factor as a function of \pt for prompt \Dp mesons integrated at the (left) forward rapidity, $2.0 < y^{*} < 4.0$, and (right) backward rapidity, $-4.5 < y^{*} < -2.5$ (right). The error bars show the statistical uncertainties and the boxes show the systematic uncertainties. The theoretical calculations are also shown \cite{Eskola:2016oht, Kovarik:2015cma, Ducloue:2015gfa, Ducloue:2016ywt, Ma:2018bax}.}
    \label{fig:RpPb_Dp_pt}
\end{figure} 

\begin{figure}[tb]
    \begin{center}
    \includegraphics[width=0.49\linewidth]{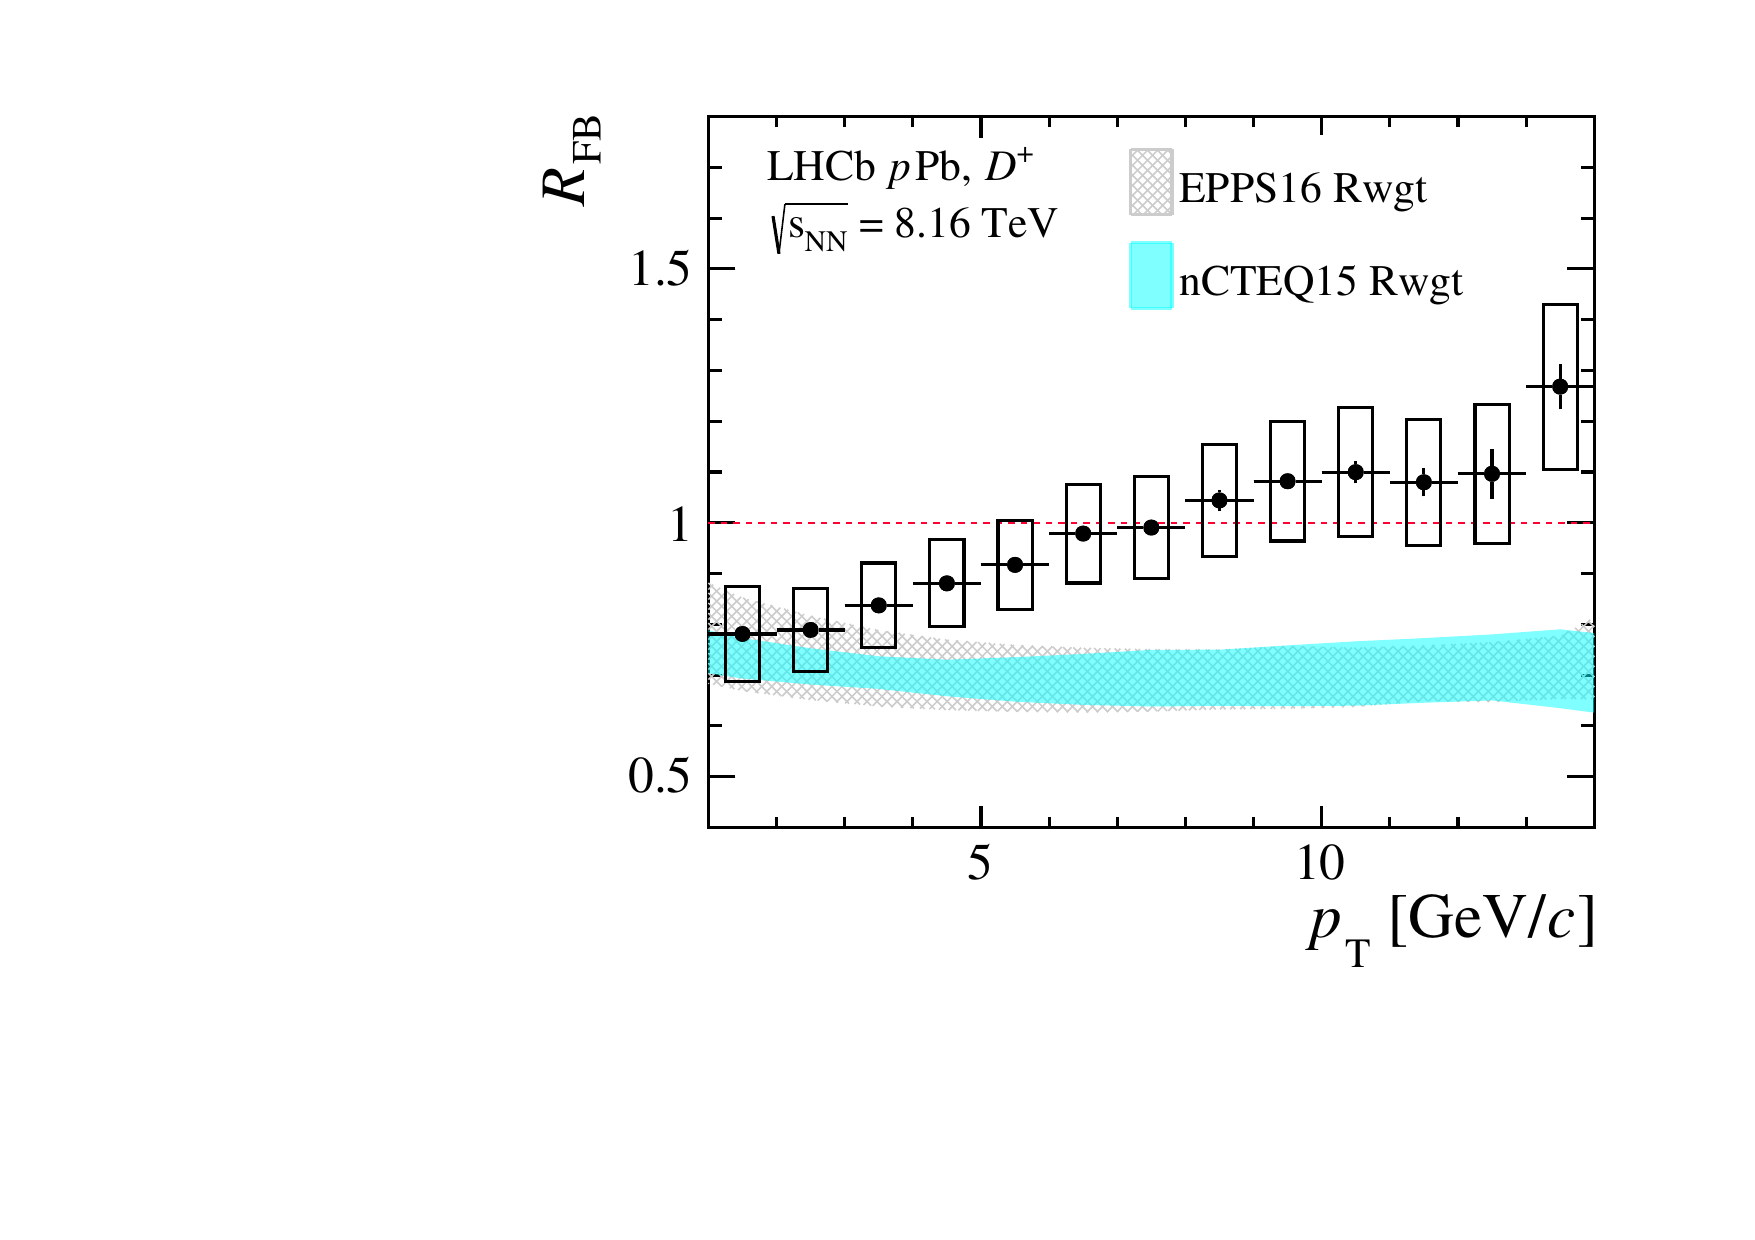}
    \includegraphics[width=0.49\linewidth]{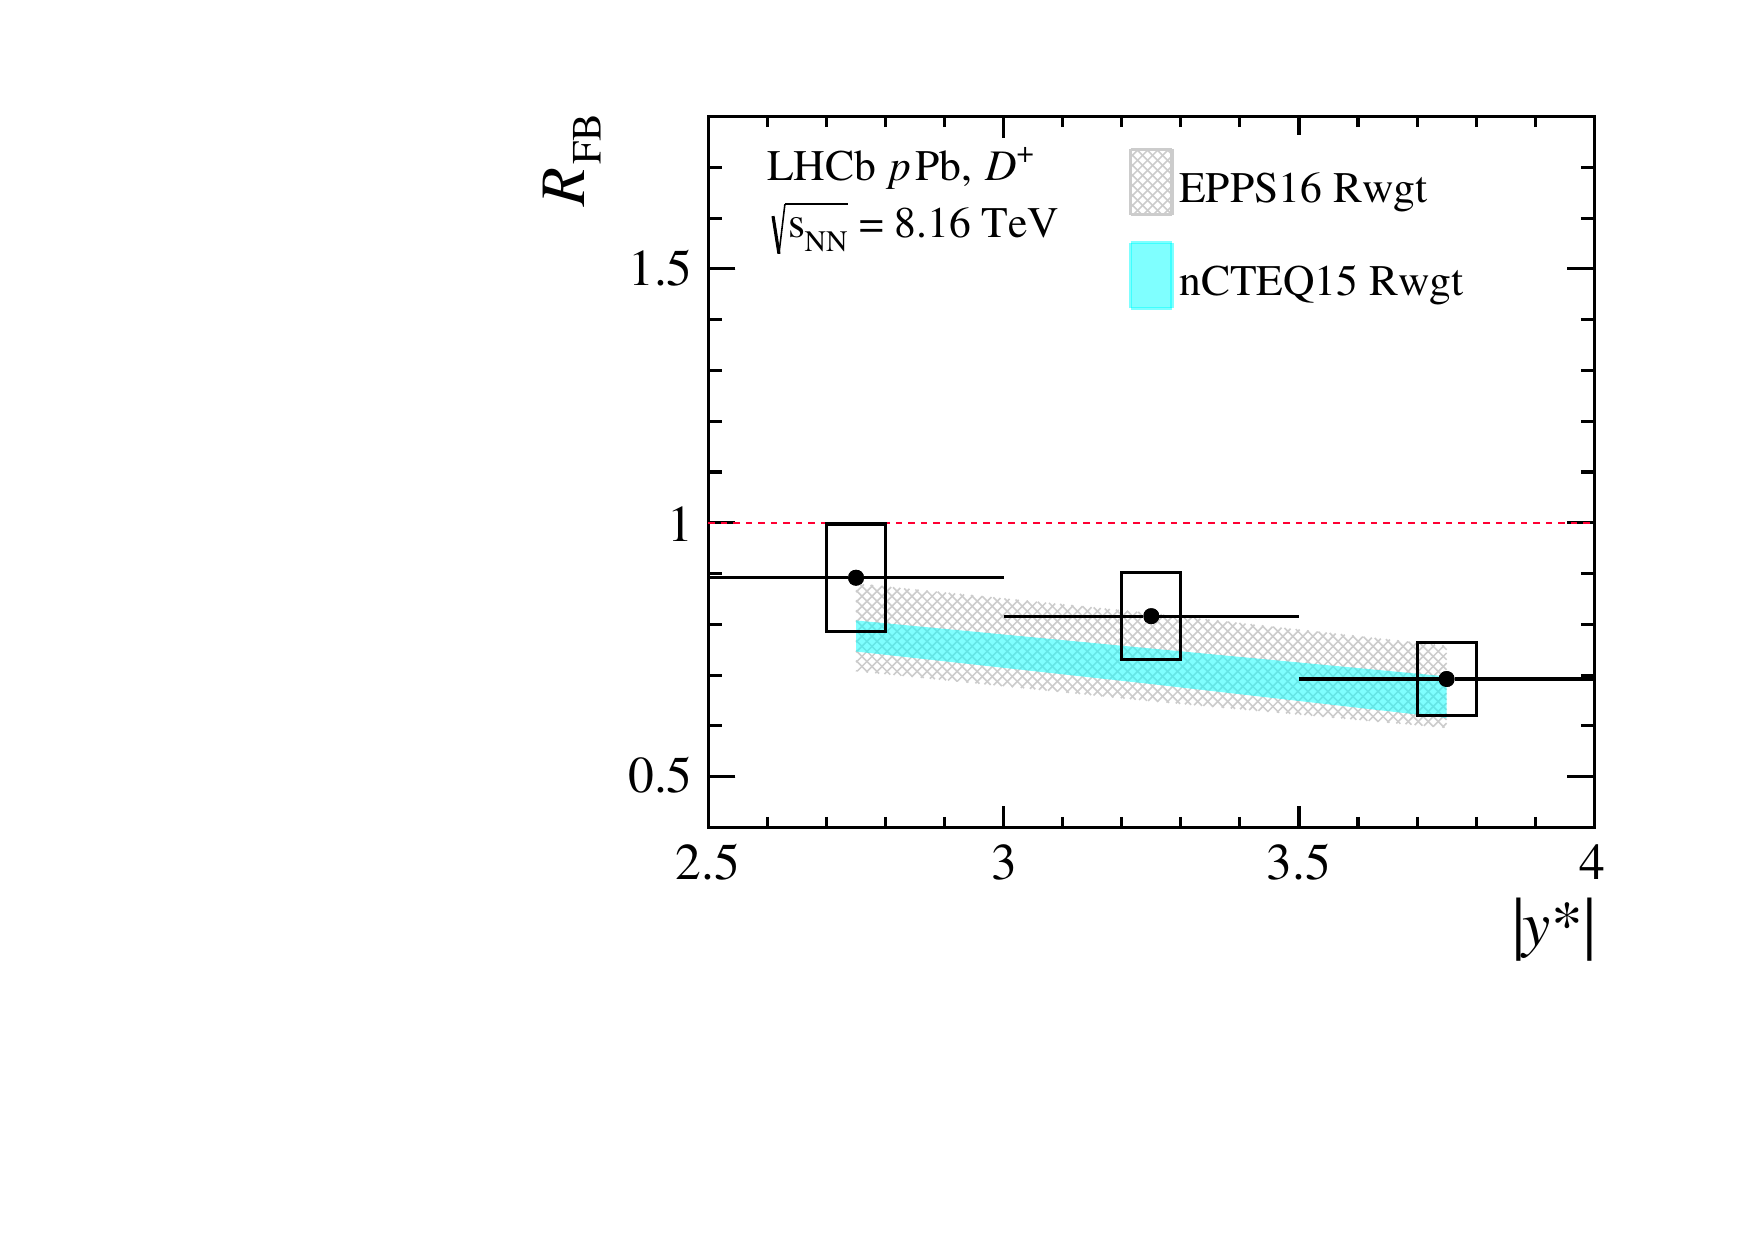}
    \vspace*{-0.5cm}
    \end{center}
    \caption{
    Forward and backward production ratio $R_{\mathrm{FB}}$ for prompt \Dp as a function of (left) \pt and (right) $y^{*}$. 
    %integrated over common rapidity and $\pt$ range : $1<\pt<13\gevc$ for $2.5 < |y^*| < 3.0$ , $1<\pt<11\gevc$ for $3.0 < |y^*| < 3.5$ , $1<\pt<7\gevc$ for $3.5 < |y^*| < 4.0$     
    The error bars are the statistical uncertainties, the boxes the systematic. The coloured bands mark the theoretical calculations, incorporating nPDFs EPPS16 (gray) \cite{Eskola:2016oht} and nCTEQ15 (cyan) \cite{Kovarik:2015cma}.}
    \label{fig:RFB_Dp}
\end{figure}

\clearpage
